# Supplementary material for: Anomalous Scaling for Hydrodynamic Lubrication of Conformal Surfaces
Source: arXiv:2306.17696 ancillary file (2023-06-30)
Supplement: Supplementary file 1 [file SM.pdf]

# Supplemental Material: Anomalous Scaling for Hydrodynamic Lubrication of Conformal Surfaces

James A. Richards,<sup>1,\*</sup> Patrick B. Warren,<sup>2,†</sup> Daniel J. M. Hodgson,<sup>1</sup> Alex Lips,<sup>1</sup> and Wilson C. K. Poon<sup>1,‡</sup>

<sup>1</sup>*Edinburgh Complex Fluids Partnership and School of Physics and Astronomy, The University of Edinburgh, James Clerk Maxwell Building, Peter Guthrie Tait Road, Edinburgh EH9 3FD, United Kingdom*

<sup>2</sup>*The Hartree Centre, STFC Daresbury Laboratory, Warrington WA4 4AD, United Kingdom*

Further experimental details for triborheological tests, including: silicone oil viscosity measurements, § S1; estimates of temperature variation, § S2; effects of rotation direction, § S3; imaging of surface details, § S4 and, axial compliance measurements, § S5.

## S1. SILICONE OIL VISCOSITIES

The nominal viscosities for the poly-dimethyl siloxane (PDMS) silicone oils, as purchased, are kinematic viscosities at 25 °C. For the Sommerfeld number we use dynamic viscosities measured at 20 °C, the test temperature for the Stribeck curves. Silicone oil viscosities were measured using a smooth cone-plate geometry [20 °C temperature, 40 mm diameter, 1° angle, Kinexus Ultra+ rheometer (Malvern, UK)]. An average of three separate runs, as single controlled-rate upsweeps at 5 pts/decade, from  $\dot{\gamma} = 1 \text{ s}^{-1}$  to  $1 \times 10^3 \text{ s}^{-1}$ , was taken to give the viscosity value used in calculating the Sommerfeld number. Inertial sample fracture occurred at higher shear rates.

The lowest viscosity oil, 5 cSt (Merck, UK, silicone oil, PDMS, 317667), was measured at 5.08(5) mPa s, Fig. S1 (triangles); we refer to this in the main text as 5 mPa s. The moderate viscosity silicone oil, 50 cSt (Merck, UK, silicone oil, PDMS, 378356), was measured at 53.2(6) mPa s, Fig. S1 (squares); we refer to this in the main text as 50 mPa s. The highest viscosity silicone oil, 500 cSt (Merck, UK, silicone oil, PDMS, 378380) was measured at 509(6) mPa s, Fig. S1 (circles); we refer to this as 500 mPa s.

Within the accessible shear rate regime, no shear thinning was observed. Although higher shear rates may be accessed

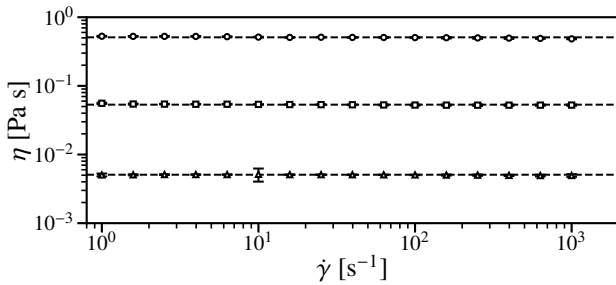

FIG. S1. Reference viscosity measurements for silicone oils. Cone-plate viscosity measurements from  $\dot{\gamma} = 1 \text{ s}^{-1}$  to  $10 \times 10^3 \text{ s}^{-1}$  for silicone oils with nominal viscosities: 5 (triangles), 50 (squares) and 500 cSt (circles). Measured viscosities, dashed lines: 5.08(5) mPa s, 53.2(6) mPa s, and 509(6) mPa s (respectively). Error bars represent standard deviation in three separate runs.

\* jamesrichards92@gmail.com

† patrick.warren@stfc.ac.uk

‡ w.poon@ed.ac.uk

during triborheological tests for the low viscosity (and low molecular weight) a Newtonian behavior is expected at all applied shear stresses [1]. For higher molecular weight silicone oils or higher shear stresses, the non-Newtonian behavior (shear thinning and normal stress differences) may need to be considered.

## S2. TEMPERATURE VARIATION

The introduction of a self-aligning plate reduces the direct thermal connection from the Peltier plate, which is used for temperature control in conventional rheological measurements. We must therefore consider whether there are significant temperature changes during the course of the experiment that might drive changes in the viscosity. During experiments the self-aligning plate and ring are contained within a solvent trap in thermal contact with the Peltier plate and equilibrated at 20 °C. This controls the initial temperature of the fluid. However, as the surfaces are sheared frictional or viscous heating may occur and we must consider whether the temperature of the fluid will rise significantly.

We must first consider if heat generated from the fluid will transfer to the plates. For a given lengthscale,  $L \sim 10 \mu\text{m}$ , a diffusive time,  $L^2/\alpha$ , can be estimated from the thermal properties of the silicone oil,  $\alpha = k/\rho c_p$  (from the thermal conductivity,  $k$ , the density,  $\rho$ , and the specific heat capacity,  $c_p$ ). Using literature values for low viscosity PDMS [2] we find  $L^2/\alpha \approx 0.001 \text{ s}$ . For experiments over 600 s, the fluid will be at the same temperature as the surface of the plates. We must now consider if the heat generated will diffuse through the aluminum plates. Over  $L \approx 1 \text{ cm}$ ,  $L^2/\alpha \sim 1 \text{ s}$  and the plate will be at a uniform temperature (using  $k = 240 \text{ W m}^{-1} \text{ K}^{-1}$ ,  $\rho = 2700 \text{ kg/m}^3$  and  $c_p = 910 \text{ J kg}^{-1} \text{ K}^{-1}$ ).

However, assessing the transfer of heat from the plate (convection via air) and the ring (conduction via rheometer shaft) is challenging. If we assume a worst case scenario, that no heat is lost from the geometry, we can estimate a maximum temperature rise in the fluid over the experiment. For this we need the thermal mass of the geometry  $\approx 100 \text{ g} \times c_p \approx 100 \text{ J K}^{-1}$  and the work done during a tribological experiment. For this we consider the total angular displacement from  $\Omega = 0.1 \text{ rad s}^{-1}$  to  $100 \text{ rad s}^{-1}$  of 3540 rad and the maximum torque limit  $\mathcal{T} = 0.05 \text{ N m}$ , so the upper limit for energy input is 180 J. This gives an upper limit for the temperature rise of  $\lesssim 2 \text{ °C}$ , neglecting any heat transfer from the geometry and that for most of the test the torque is far below the maximum limit.

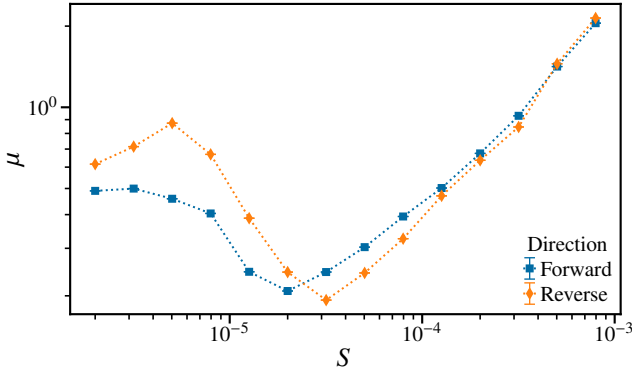

FIG. S2. Stribeck curve from tribo-rheology for forward [(blue) squares] and reverse [(orange) diamonds] rotation at  $N = 0.5$  N and  $\eta = 50$  mPa s.

As silicone oils are widely used due to their low sensitivity to changes in temperature, we consider the temperature to be constant with regards to changes in viscosity.

### S3. REVERSIBILITY OF MEASUREMENTS

As the surface profile is approximately symmetrical (for different directions of motion), Fig. 3 (upper inset), we should observe comparable Stribeck curves for opposite directions of motion (experimentally, positive and negative  $\Omega$ ). Noting here that the lift is only produced in the converging gap and that the converging and diverging parts of the profile switch positions on reversal. In Fig. S2, the forward direction [(blue) squares] and reverse [(orange) diamonds] show similar behavior. In the high  $S$  limit they are near equivalent, where the only parameters of relevance are  $d$  and  $D$ , *i.e.* where the behavior is most insensitive to the surface profile, which are similar for the forward and reverse directions, Fig. 3 (upper inset). As  $S$  decreases towards the point of deviation, we see a small difference which may reflect the slight change in  $D$  (as the surface profile is not completely symmetric to reversal). At the lowest we observe a significant difference, here the detailed surface profile may come into play as the surfaces approach and, at the lowest  $S$ , contact. For a highly asymmetric surface profile the behavior on reversal would not be expected to show such invariance.

### S4. SURFACE ROUGHNESS IMAGING

In the main text the full circumferential profile of the surfaces was characterised using a rheometer as a surface probe, Fig. 4 (upper inset). However, with the surfaces as machined there may also surface texturing in the radial direction. This was probed using confocal microscopy to image the surface profile in a selected region. The ring or plate was placed above a coverslip on an inverted confocal microscope [Leica SP8, 10 $\times$ (0.3) dry objective] with a layer of fluorescently dyed solution [88 wt% glycerol (Fisher Scientific, UK) with water and

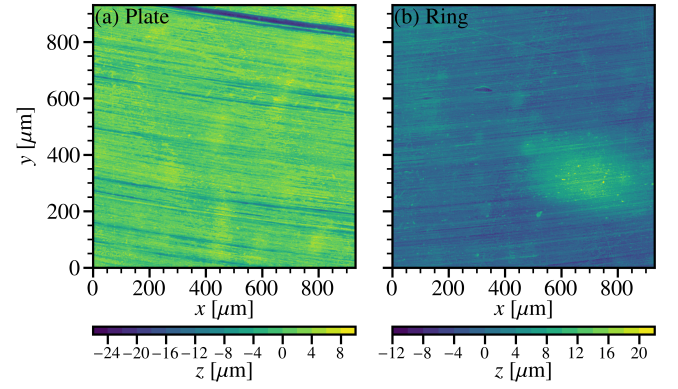

FIG. S3. Qualitative surface topography of tribo-rheology surfaces from confocal microscopy. (a) Plate surface height  $z(x, y)$ , see corresponding lower colorbar. (b) Ring surface.

0.2 mM sodium fluorescein salt (Merck, UK)]. With excitation wavelength  $\lambda = 488$  nm, three-dimensional 8-bit images were taken at  $1024 \times 1024$  px<sup>2</sup> with  $0.91 \mu\text{m}$  pixel resolution and  $2.4 \mu\text{m}$   $z$  spacing (based on  $z$  resolution with reduced pinhole diameter of 0.4 Airy units) for emission wavelengths 500 nm to 600 nm. To produce a surface topography the image is thresholded based on the pixel histogram, binarised, averaged over  $z$ , inverted and the tilt (from placing on the coverslip) is removed, Fig. S3.

The plate, Fig. S3a, shows striations in the flow direction, *i.e.* patterning consistent with rotary machining. Although the peak amplitude is large this arises from *indents* into the surface. The average root mean square roughness over the imaged region is  $3.3 \mu\text{m}$ , consistent with the circumferential profile. Similarly, the ring also displayed (finer) striations consistent with machining with roughness  $3.0 \mu\text{m}$ , where diffuse feature with a positive height appears due to an imaging artefact. To fully characterise the radial patterning and surface profile of the geometry would require a scan of comparable resolution across the whole geometry, *i.e.* centimetre scales. The results from this limited surface profiling suggest the presence of radial patterning of a lengthscale as invoked in the main article, *i.e.* less than (but comparable in order of magnitude) to the  $20 \mu\text{m}$  circumferential undulations.

### S5. COMPLIANCE

A possible explanation of the load dependent lubrication, *i.e.* ‘spurious EHL’, in which the deviation point from the  $\mu \sim S^{2/3}$  scaling,  $S^*$ , shifts to lower  $S$  would be a decreasing  $d$ . A 10-fold decrease in  $S^*$  over the range  $N = 0.1$  to  $1.0$  N (dark purple to light green in Fig. 4) suggests  $d/L \sim \sqrt{S^*}$  decreases by a factor of  $\sqrt{10}$ , Eq. (1). Changing  $L$  would require rather unlikely bulk deformations. However, uneven support of the ring’s upper surface by the plate to which it is attached, *e.g.*, due to machining undulations (Fig. 4, upper inset), could give deflections  $\Delta d \sim FR^2/EI$ . With  $E = 70$  GPa and  $I = Lt^3/12$  for thickness  $t = 4$  mm,  $\Delta d \sim 20 \mu\text{m}$ , which could explain the

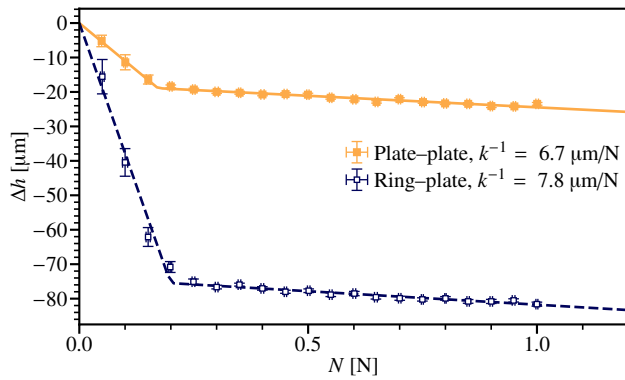

FIG. S4. Compliance of triborheology geometry. Vertical deformation,  $\Delta h$ , with increasing normal load,  $N$ . Symbols: light (orange), deformation with upper parallel plate and lower self-aligning plate; dark (blue), upper ring geometry mounted to plate. Lines, fit of piecewise linear spring model for low force alignment from tilting of lower plate and high force axial compliance. Reported values of compliance,  $k^{-1}$ , are for  $N \gtrsim 0.2$  N.

shift.

Experimental measurement of the axial compliance was performed by application of a fixed normal load upon the self-aligning tribo-rheology geometry from 0.05 N to 1.0 N and measurement of the reported decrease in the gap,  $\Delta h$ . By comparing the compliance without the ring,  $k^{-1} = 6.7 \mu\text{m N}^{-1}$  [Fig. S4 (light orange), axial loading, force transmission from upper cone geometry directly to lower plate], and with the ring,  $k^{-1} = 7.8 \mu\text{m N}^{-1}$  [Fig. S4 (dark blue), ring loading] the compliance of the ring itself can be estimated  $k^{-1} = 1.1 \mu\text{m N}^{-1}$ . This is an order of magnitude less than the required compliance, suggesting that the ring is well supported. The primary contributor to the compliance is the bearing of the rheometer, but note that this does not influence the constant normal force tests used in the main text. It should also be noted that the test is static (non-rotating) and unlubricated compression, in contrast to the conditions for tribo-rheology. As such, the minimum force for alignment given by the transition from the high compliance of the foam to the bearing compliance,  $\sim 0.2$  N, is larger and not comparable to results in Fig. 4.

[1] R. Weijermars, Polydimethylsiloxane flow defined for experiments in fluid dynamics, *Appl. Phys. Lett.* **48**, 109 (1986).

[2] J. E. Mark, *The Polymer Data Handbook* (Oxford University Press, 1999).
